# Supplementary material for: Preacher: Paper-to-Video Agentic System
Source: arXiv:2508.09632 source file (2025-09-08)
Supplement: Supplementary file 1 [file 7_appendix.tex]

\newpage
\section{Benchmark}
\label{sec_7_B}
We choose papers from 5 fields:Mathematics, Molecular Biology, Geology, Machine Learning, and Climate Science. The paper list is shown below:

Mathematics:
\textit{``Solutions of irreflexive relations''} by Richardson M. (1953),  \textit{``On the existence of hermitian-yang-mills connections in stable vector bundles''} by Uhlenbeck,K. and Yau,S. T. (1985), \textit{``Higher algebraic structures and quantization''} by Freed D S. (1994), \textit{`` Understanding qualitative calculus:A structural synthesis of learning research''} by Stroup W M. (2002), \textit{``Oscillation theorems in the complex domain''} by Hille E.  (1922), \textit{``Fourier integral operators.''} by Hörmander L. (1971), \textit{``Solutions of irreflexive relations''} by Richardson M. (1953), \textit{``Internal set theory:a new approach to nonstandard analysis''} by Nelson E. (1977), \textit{``Topological vector spaces of continuous functions''} by Nachbin L.  (1954), \textit{``Oscillation theory''} by Kreith K. (1973)

Molecular Biology:
\textit{``Molecular structure of nucleic acids:a structure for deoxyribose nucleic acid''} by Watson J D, Crick F H C (1953),  \textit{``DNA sequencing at 40:past, present and future''} by Shendure J, Balasubramanian S, Church G M, et al. (2017),  \textit{``Specific enzymatic amplification of DNA in vitro:the polymerase chain reaction''} by Mullis K, Faloona F, Scharf S, et al. (1986),  \textit{``C2c1-sgRNA complex structure reveals RNA-guided DNA cleavage mechanism''} by  Liu L, Chen P, Wang M, et al. (2017), \textit{``C2c1-sgRNA complex structure reveals RNA-guided DNA cleavage mechanism''} by Liu L, Chen P, Wang M, et al. (2017),  \textit{``An archaeal CRISPR type III-B system exhibiting distinctive RNA targeting features and mediating dual RNA and DNA interference''} by Peng W, Feng M, Feng X, et al. (2015),  \textit{``Meningioma:International Consortium on Meningiomas consensus review on scientific advances and treatment paradigms for clinicians, researchers, and patients''} by Wang J Z, Landry A P, Raleigh D R, et al. (2024),  \textit{``Imaging live-cell dynamics and structure at the single-molecule level''} by Liu Z, Lavis L D, Betzig E.  (2015), \textit{``Genetic regulatory mechanisms in the synthesis of proteins''} by  Jacob F, Monod J. (1961), \textit{``Aquaporins in plants''} by Maurel C, Boursiac Y, Luu D T, et al. (2015) 

Geology:
\textit{``Effects of cattle husbandry on abundance and activity of methanogenic archaea in upland soils''} by Radl V, Gattinger A, Chroňáková A, et al. (2007), 
\textit{``Proterozoic to Phanerozoic case studies of laser ablation microanalysis for microbial carbonate U–Pb geochronology''} by Jiang Y, Hohl S V, Huang X, et al.  (2024), 
\textit{``Zircon $U–Pb$ ages and $O–Hf$ isotopes of Quaternary trachytes from the East Sea: Implications for the genesis of low-$\delta$18O magmas''} by Choi H O, Oh J, Kim C H, et al. (2024), 
\textit{``Fluoride contamination in groundwater: A global review of the status, processes, challenges, and remedial measures''} by Shaji, E., et al.  (2024), 
\textit{``Metagenomic insights into soil microbial communities under climate change''} by Elhottova, D., et al. (2023), 
\textit{``Molecular biomarkers in ancient sediments:Tracking microbial evolution through deep time''} by Huang, X., et al. (2022), 
\textit{``Meningioma:International Consortium consensus review on molecular classification''} by Wang, J.Z., et al. (2024), 
\textit{``Real-time visualization of single-molecule transcription dynamics''} by Hoskins, A.A., et al.  (2024), 
\textit{``Nanoscale mineral-fluid interactions:Implications for carbon sequestration''} by Kim,C.H, et al.  (2023), 
\textit{``Cosmochemical constraints on the sulfur content in the Earth's core''} by Dreibus G, Palme H. (1996), 
\textit{``A reinforced lunar dynamo recorded by Chang'e-6 farside basalt''} by Shuhui Cai, et al. (2024),

Machine Learning:
\textit{``Syntactic representations of semantic merging operations''} by Meyer T, Ghose A, Chopra S.  (2002),
\textit{``Artificial intelligence in medicine''} by Holmes J, Sacchi L, Bellazzi R.  (2004),
\textit{``Adding conditional control to text-to-image diffusion models''} by Zhang L, Rao A, Agrawala M.  (2023),
\textit{``Evaluation of the use of combined artificial intelligence and pathologist assessment to review and grade prostate biopsies''} by Steiner D F, Nagpal K, Sayres R, et al. (2000),
\textit{``Erasing concepts from diffusion models''} by Gandikota R, Materzynska J, Fiotto-Kaufman J, et al. (2023),
\textit{``Explainable AI over the Internet of Things (IoT):Overview, state-of-the-art and future directions''} by Jagatheesaperumal S K, Pham Q V, Ruby R, et al.  (2022),
\textit{`` Exploring the potential of GPT-4 in biomedical engineering:the dawn of a new era''} by Cheng K, Guo Q, He Y, et al. (2023),
\textit{``Blockchain technology in financial sector and its legal implications''} by Divyashree K S, Mishra A. (2022),
\textit{``Artificial intelligence in education''} by Moturu V R, Nethi S D.  (2022),
\textit{``Automated haggling:Building artificial negotiators''} by Jennings N R, Faratin P, Lomuscio A R, et al.  (2000),

Climate Science:
\textit{``Global warming in the pipeline''} by Hansen J E, Sato M, Simons L, et al.  (2023),
\textit{``Possible seismogenic-trigger mechanism of methane emission, glacier destruction and climate warming in the Arctic and Antarctic''} by Lobkovsky L I, Baranov A A, Ramazanov M M, et al. (2023),
\textit{``Temperature, crime, and violence:A systematic review and meta-analysis[J]. Environmental Health Perspectives''} by Choi H M, Heo S, Foo D, et al.  (2024),
\textit{``The missing risks of climate change''} byRising J, Tedesco M, Piontek F, et al.  (2022),
\textit{``Climate change 2022:Mitigation of climate change''} by Shukla P R, Skea J, Slade R, et al.  (2022),
\textit{``Informing decisions in a changing climate''} by National Research Council, Division of Behavioral, Social Sciences, et al. (2009),
\textit{``The impact of the permafrost carbon feedback on global climate''} by Schaefer K, Lantuit H, Romanovsky V E, et al. (2014),
\textit{``Permafrost carbon-climate feedbacks accelerate global warming''} by Koven C D, Ringeval B, Friedlingstein P, et al. (2011),
\textit{``Global climate change:the potential effects on health''} by McMichael A J, Haines A. (1997),
\textit{``The human imperative of stabilizing global climate change at 1.5 C''} by Hoegh-Guldberg O, Jacob D, Taylor M, et al. (2019),

\begin{figure}[h]
\centering
\includegraphics[width=0.99\linewidth]{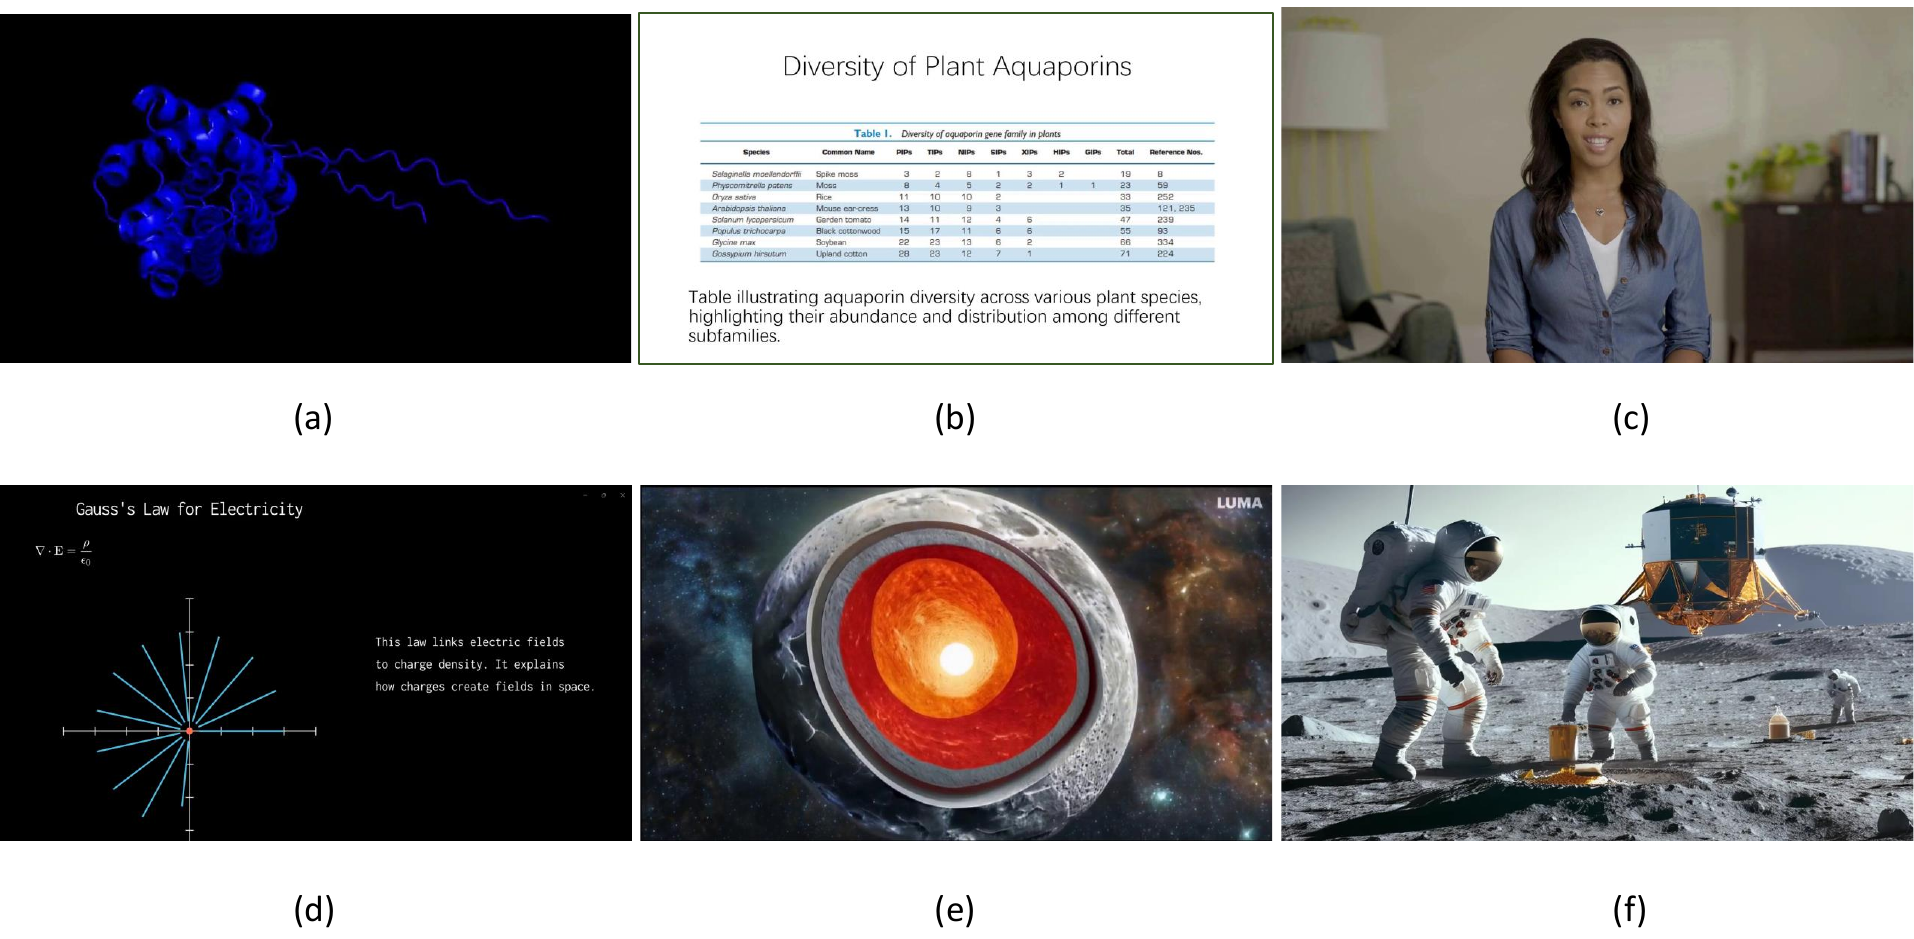}
\vspace{-0.07in}
\caption{Preacher can generate video abstracts with six different video styles. (a) Molecular Visualization (b) Slides (c) Talking Heads, (d) Mathematics, (e) General Style (f) Static concept.} 
\vspace{-0.5em}
\label{fig:st}
\vspace{-0.07in}
\end{figure}

\section{More Details of Preacher}
\subsection{Different Styles of Video Abstract}
\label{sec_7_VS}
A video abstract is a specialized format of video content in which a single video abstract can integrate multiple distinct styles concurrently \citep{gupta2021integrated}. Preacher currently supports the generation of six such styles: ``talking heads,'' ``general style,'' ``static concept,'' ``molecular visualization,'' ``slides,'' and ``mathematics.'', as shown in \cref{fig:st}. Below is a detailed introduction and implementation methodology for each video style:

\textit{Molecular Visualization}
Biological and chemical research papers often include discussions on specific molecular structures. Visualizing these structures enhances reader comprehension by providing a clear representation of complex molecular configurations. We employ pymol=3.0.0 to generate three-dimensional molecular structures from multiple perspectives, which are then compiled into a cohesive video. Given the access restrictions on repositories such as AlphaFold \citep{jumper2021highly}, our approach requires users to manually download the PDB (Protein Data Bank) files specified by name in the key scene for processing.

\textit{Mathematics} 
Many scientific papers contain critical formulas and theorems. Animating these mathematical principles facilitates deeper conceptual understanding. We utilize Manim = 0.18.1 for generating mathematical demonstrations. Notably, this process is highly susceptible to execution errors caused by code interruptions. To ensure robustness, we predefine a complete script and limit the AI agent’s modifications strictly to animation-related functions. Updates to the code are applied through text replacement rather than full script regeneration, significantly improving execution stability and accuracy.

\textit{Static Concept}
Certain papers introduce fundamental real-world concepts that lack intrinsic dynamism. For these, we employ wan-2.1-t2i-turbo \citep{tywx} to generate high-fidelity static visualizations, which are subsequently expanded into video sequences to enhance engagement.

\textit{General Style}:
Some abstract or complex concepts in academic literature are best conveyed through dynamic visual representation. We utilize Luma \citep{luma} to generate high-quality, contextually relevant visual content for these concepts.

\textit{Slides}
Key research findings, such as structured tables and framework diagrams, are indispensable elements of academic papers. We present these elements using a structured slide-based format with python-pptx = 1.0.2, leveraging a standardized slide template where textual and visual content is dynamically replaced to match the specific paper. To extract relevant figures, our agent identifies coordinates based on ``source'' components within the key scene and captures screenshots from the designated page accordingly. However, this automated process may be prone to errors due to planning errors from LMMs. To mitigate potential failures, users can manually capture and place the necessary images in the designated location to facilitate seamless content generation by Preacher.

\textbf{Talking Head}
The Talking Head style facilitates the articulate presentation of key insights through human narration, enhancing audience engagement and comprehension. The Talking Head style allows for the delivery of key insights through human narration. For enhanced presentation quality, we leverage a professional talking head generation API, Tavus \citep{tavus}, which enables the synthesis of high-fidelity facial animations synchronized precisely with the provided audio. This ensures realistic and articulate video outputs with accurate lip-syncing.

\begin{figure*}[ht]
\centering
\includegraphics[width=0.95\linewidth]{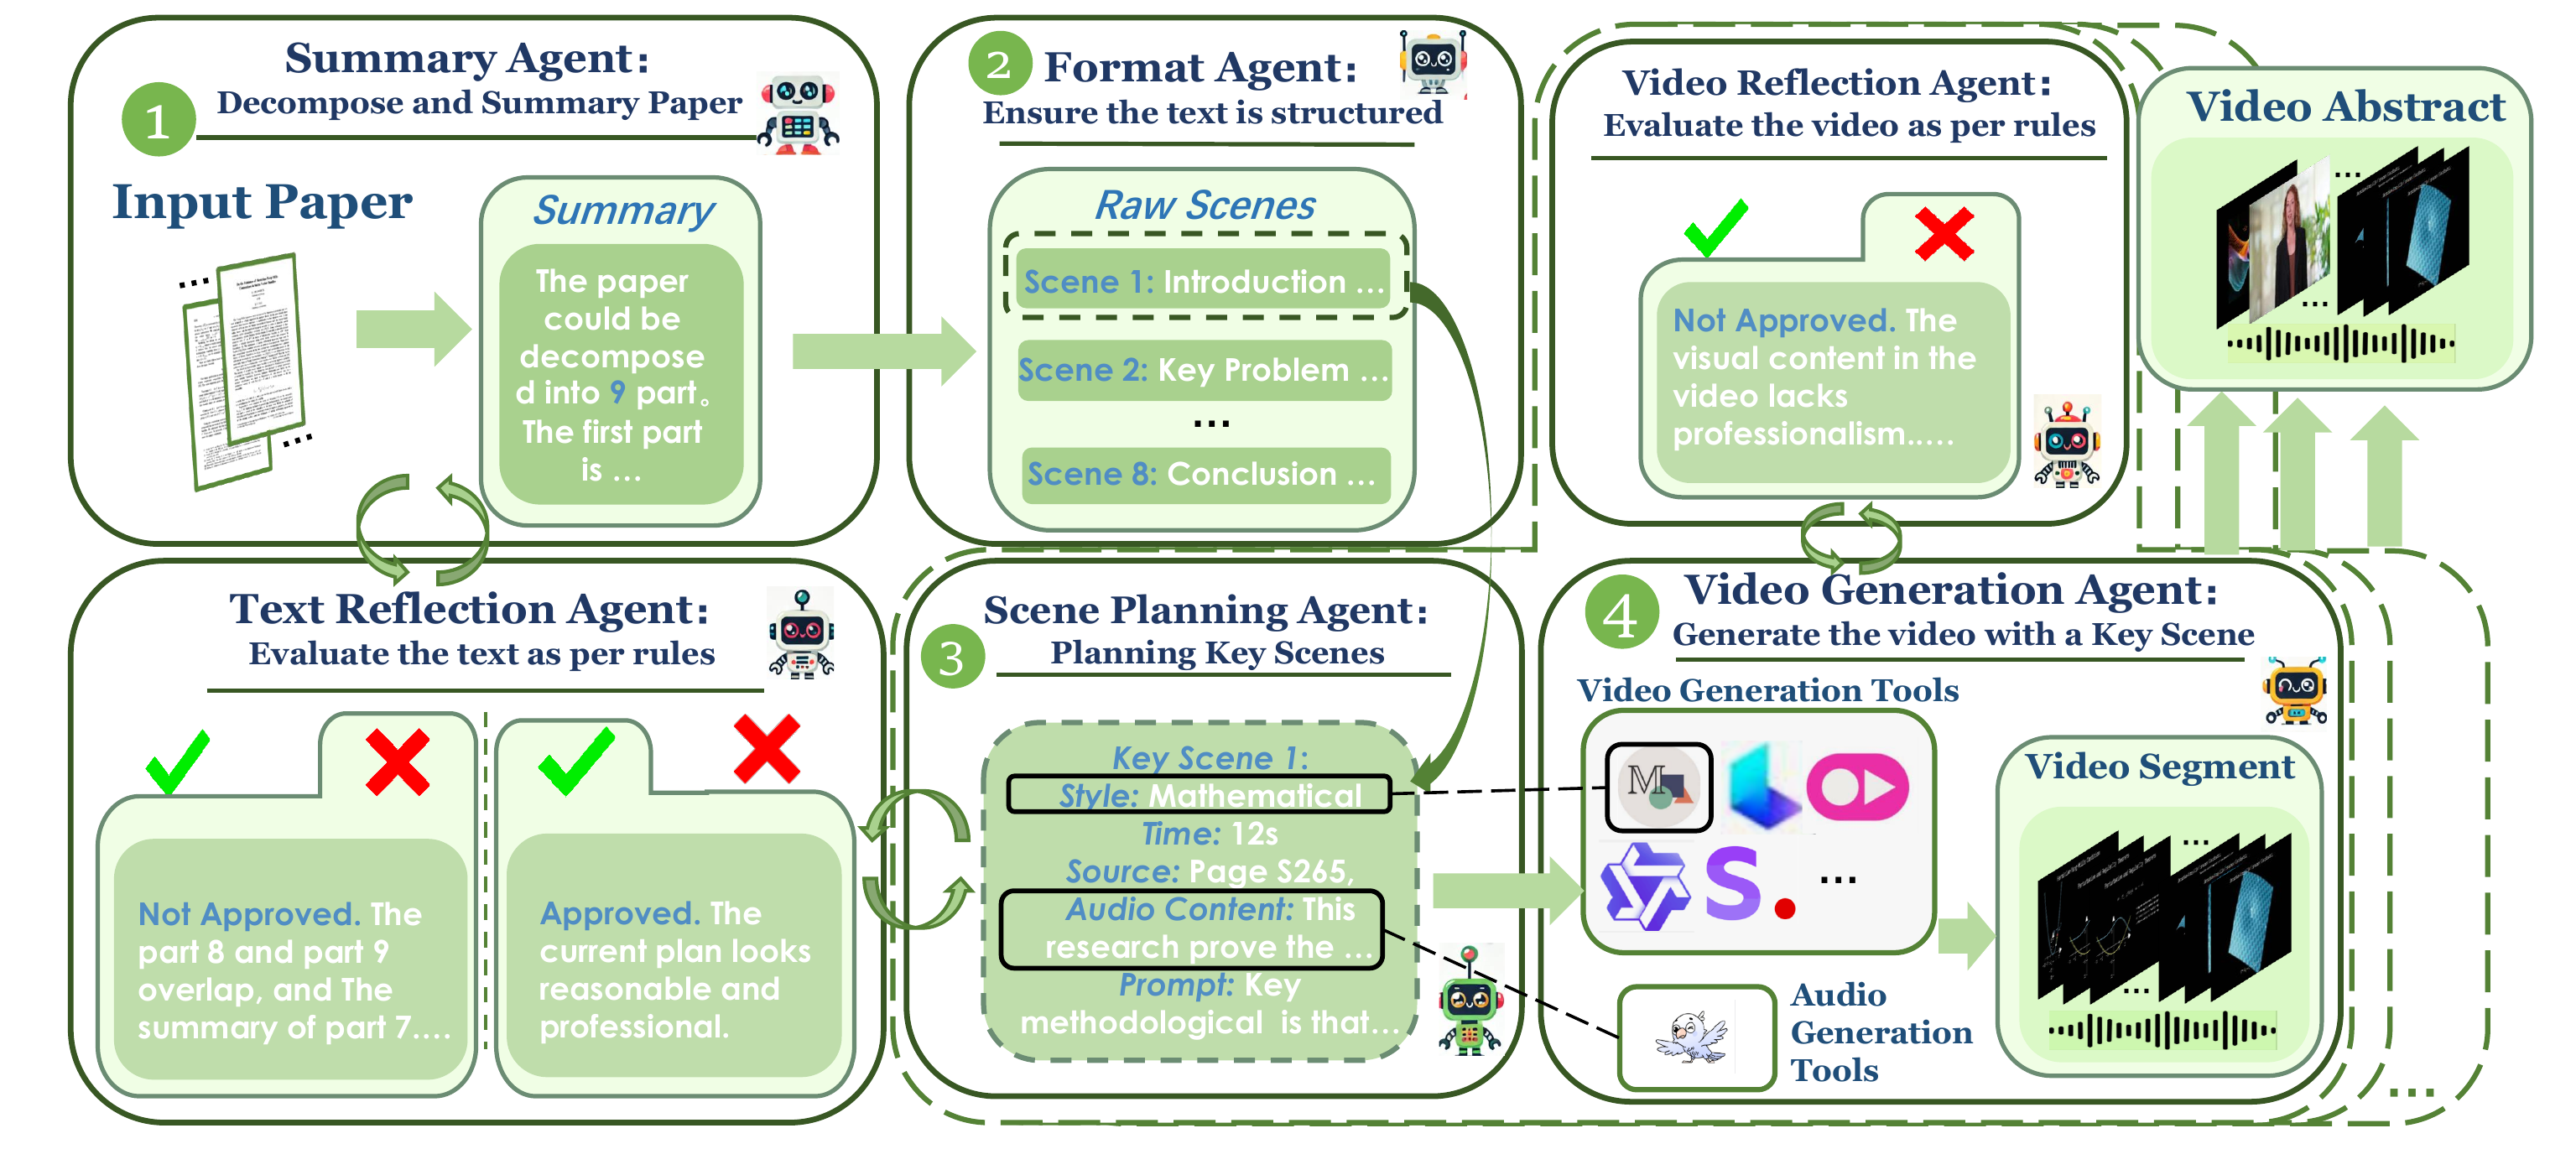}
\vspace{-0.07in}
\caption{The workflow of Preacher. The parts within the dashed box correspond to the process of generating a video segment. If the number of key scenes is $N$ scenes, the process within the dashed box will repeat $N$ times until all video segments are generated. Finally, all the video segments are concatenated as the video abstract.}
% \vspace{-0.17in}
\label{fig:workflow}
\end{figure*}

\subsection{Design of Rule-Based Reflection Agents}
\label{sec_7_r} 
Many existing multi-agent frameworks incorporate reflection mechanisms to prevent agents from generating erroneous outcomes \citep{park2023generative, shinn2023reflexion,zhangbuilding}. Preacher includes two reflection agents:the Text Reflection Agent $\mathcal{A}_{tref}$ and the Video Reflection Agent $\mathcal{A}_{vref}$. Both agents are equipped with MLMMs but serve distinct tasks. $\mathcal{A}_{tref}$ is responsible for reviewing the input paper and providing a reflection on the current plan. While $\mathcal{A}_{vref}$ evaluates keyframes in the video and compares them with the corresponding part of the paper, offering a reflection on the visual content.

Unlike other work \citep{park2023generative, shinn2023reflexion,zhangbuilding}, the task faced by Preacher is fixed. Therefore we have build specific rules to guide $\mathcal{A}_{tref}$ and $\mathcal{A}_{vref}$ in conducting targeted checks on the current content. Depending on the different planning stages and video styles, $\mathcal{A}_{tref}$ and $\mathcal{A}_{vref}$ will ask questions with different parts of the rules. These questions primarily focus on the correctness, professionalism, and consistency with the paper. We continuously update these rules throughout the practical process.%, and some of the rules are show.

\subsection{Complete Workflow}
\label{sec_7_WF}

\cref{fig:workflow} illustrates Preacher’s workflow, with the video generation process detailed in \cref{fig:trick}. After generating video segments, the corresponding audio track is synthesized based on the “audio content” in the key scenes.

Since the video duration, audio length, and predefined “time cost” in key scenes may not align, we adjust video playback speed—either slowing down or accelerating—to match the designated time cost. However, modifying audio speed introduces distortion. To mitigate this, we constrain audio script length during planning and introduce intentional pauses when the audio is shorter than required.

\section{Model Selection}
\label{sec_7_MS}

\begin{table}[!ht]
    \small
    \centering
    \caption{Performance comparisons on key scenes on four metrics. We report mean values and standard error. The best is in bold.}
    \resizebox{0.49\textwidth}{!}{
    \label{tab:app}
    \begin{tabular}{l|cccc}
    \toprule
    \textsc{\textbf{Method}} & 
     \textbf{Accuracy}$\uparrow$ & \textbf{Professionalism}$\uparrow$  & \textbf{Compatibility}$\uparrow$  & \textbf{Aliment}$\uparrow$ \\
    \midrule
    Gemini-2.0-flash & 4.70(0.35) & 4.63(0.34) & 4.38(0.66) & \textbf{4.50}(0.31) \\
    GPT-4o \citep{zheng2023chatgpt} & 4.55(0.41) & 4.30(0.61) & 4.45(0.41) & 4.40(0.61) \\
    OpenAI-o3-mini \citep{O3} & \textbf{4.80}(0.12) & 4.61(0.38) & \textbf{4.50}(0.36) & \textbf{4.50}(0.43) \\
    DeepSeek-R1\citep{deepseekai2025deepseekr1incentivizingreasoningcapability}  & \textbf{4.80}(0.14) & \textbf{4.70} (0.19) & 3.90(1.12) & 4.08(0.91) \\
    \bottomrule
    \end{tabular}
    \vspace{-0.07in}
}
\end{table}
\vspace{-0.07in}
The integration of Gemini \citep{team2023gemini} within Preacher is primarily driven by its API support for direct PDF uploads. To isolate this factor, we conducted experiments where PDFs were manually uploaded via a web interface, and prompts were entered manually. This enabled the replacement of Gemini with alternative MLMMs, allowing a systematic evaluation of their key scene planning performance. As shown in \cref{tab:app}, OpenAI-o3-mini exhibited the most consistent and effective performance. In contrast, DeepSeek generated highly precise yet overly intricate outputs, often deviating from the core content of the input paper. Given that Preacher is model-agnostic, its capabilities are expected to scale with advancements in MLMM performance and interoperability.
To further assess Preacher’s effectiveness, we directly input key scenes into state-of-the-art (SOTA) video generation models, including Wan-2.1-14B \citep{tywx} (open-source) and Sora \citep{openai2024sora} (closed-source). \cref{fig:appshow} compares the video segments generated by Preacher, Wan-2.1-14B, and Sora.

General video generation models like Sora prioritize visual continuity and aesthetic appeal but lack the ability to visualize specialized professional content. In \cref{fig:appshow}(a), existing methods fail to represent the concept of "stable bundles" and omit critical mathematical proofs. In \cref{fig:appshow}(b), while Sora and Wan attempt to depict "molecular mechanisms," they generate nonexistent cellular structures, misrepresenting the original research.
Such inaccuracies significantly diminish the scholarly value of the video abstract. By incorporating multidimensional planning, multi-stage reflective mechanisms, and diverse video generation tools, Preacher ensures an accurate and domain-specific representation of the input paper, preventing the propagation of erroneous knowledge in generated videos.

%\section{More Examples}
\label{sec_7_M}
\begin{figure*}[ht]
\centering
\includegraphics[width=0.95\linewidth]{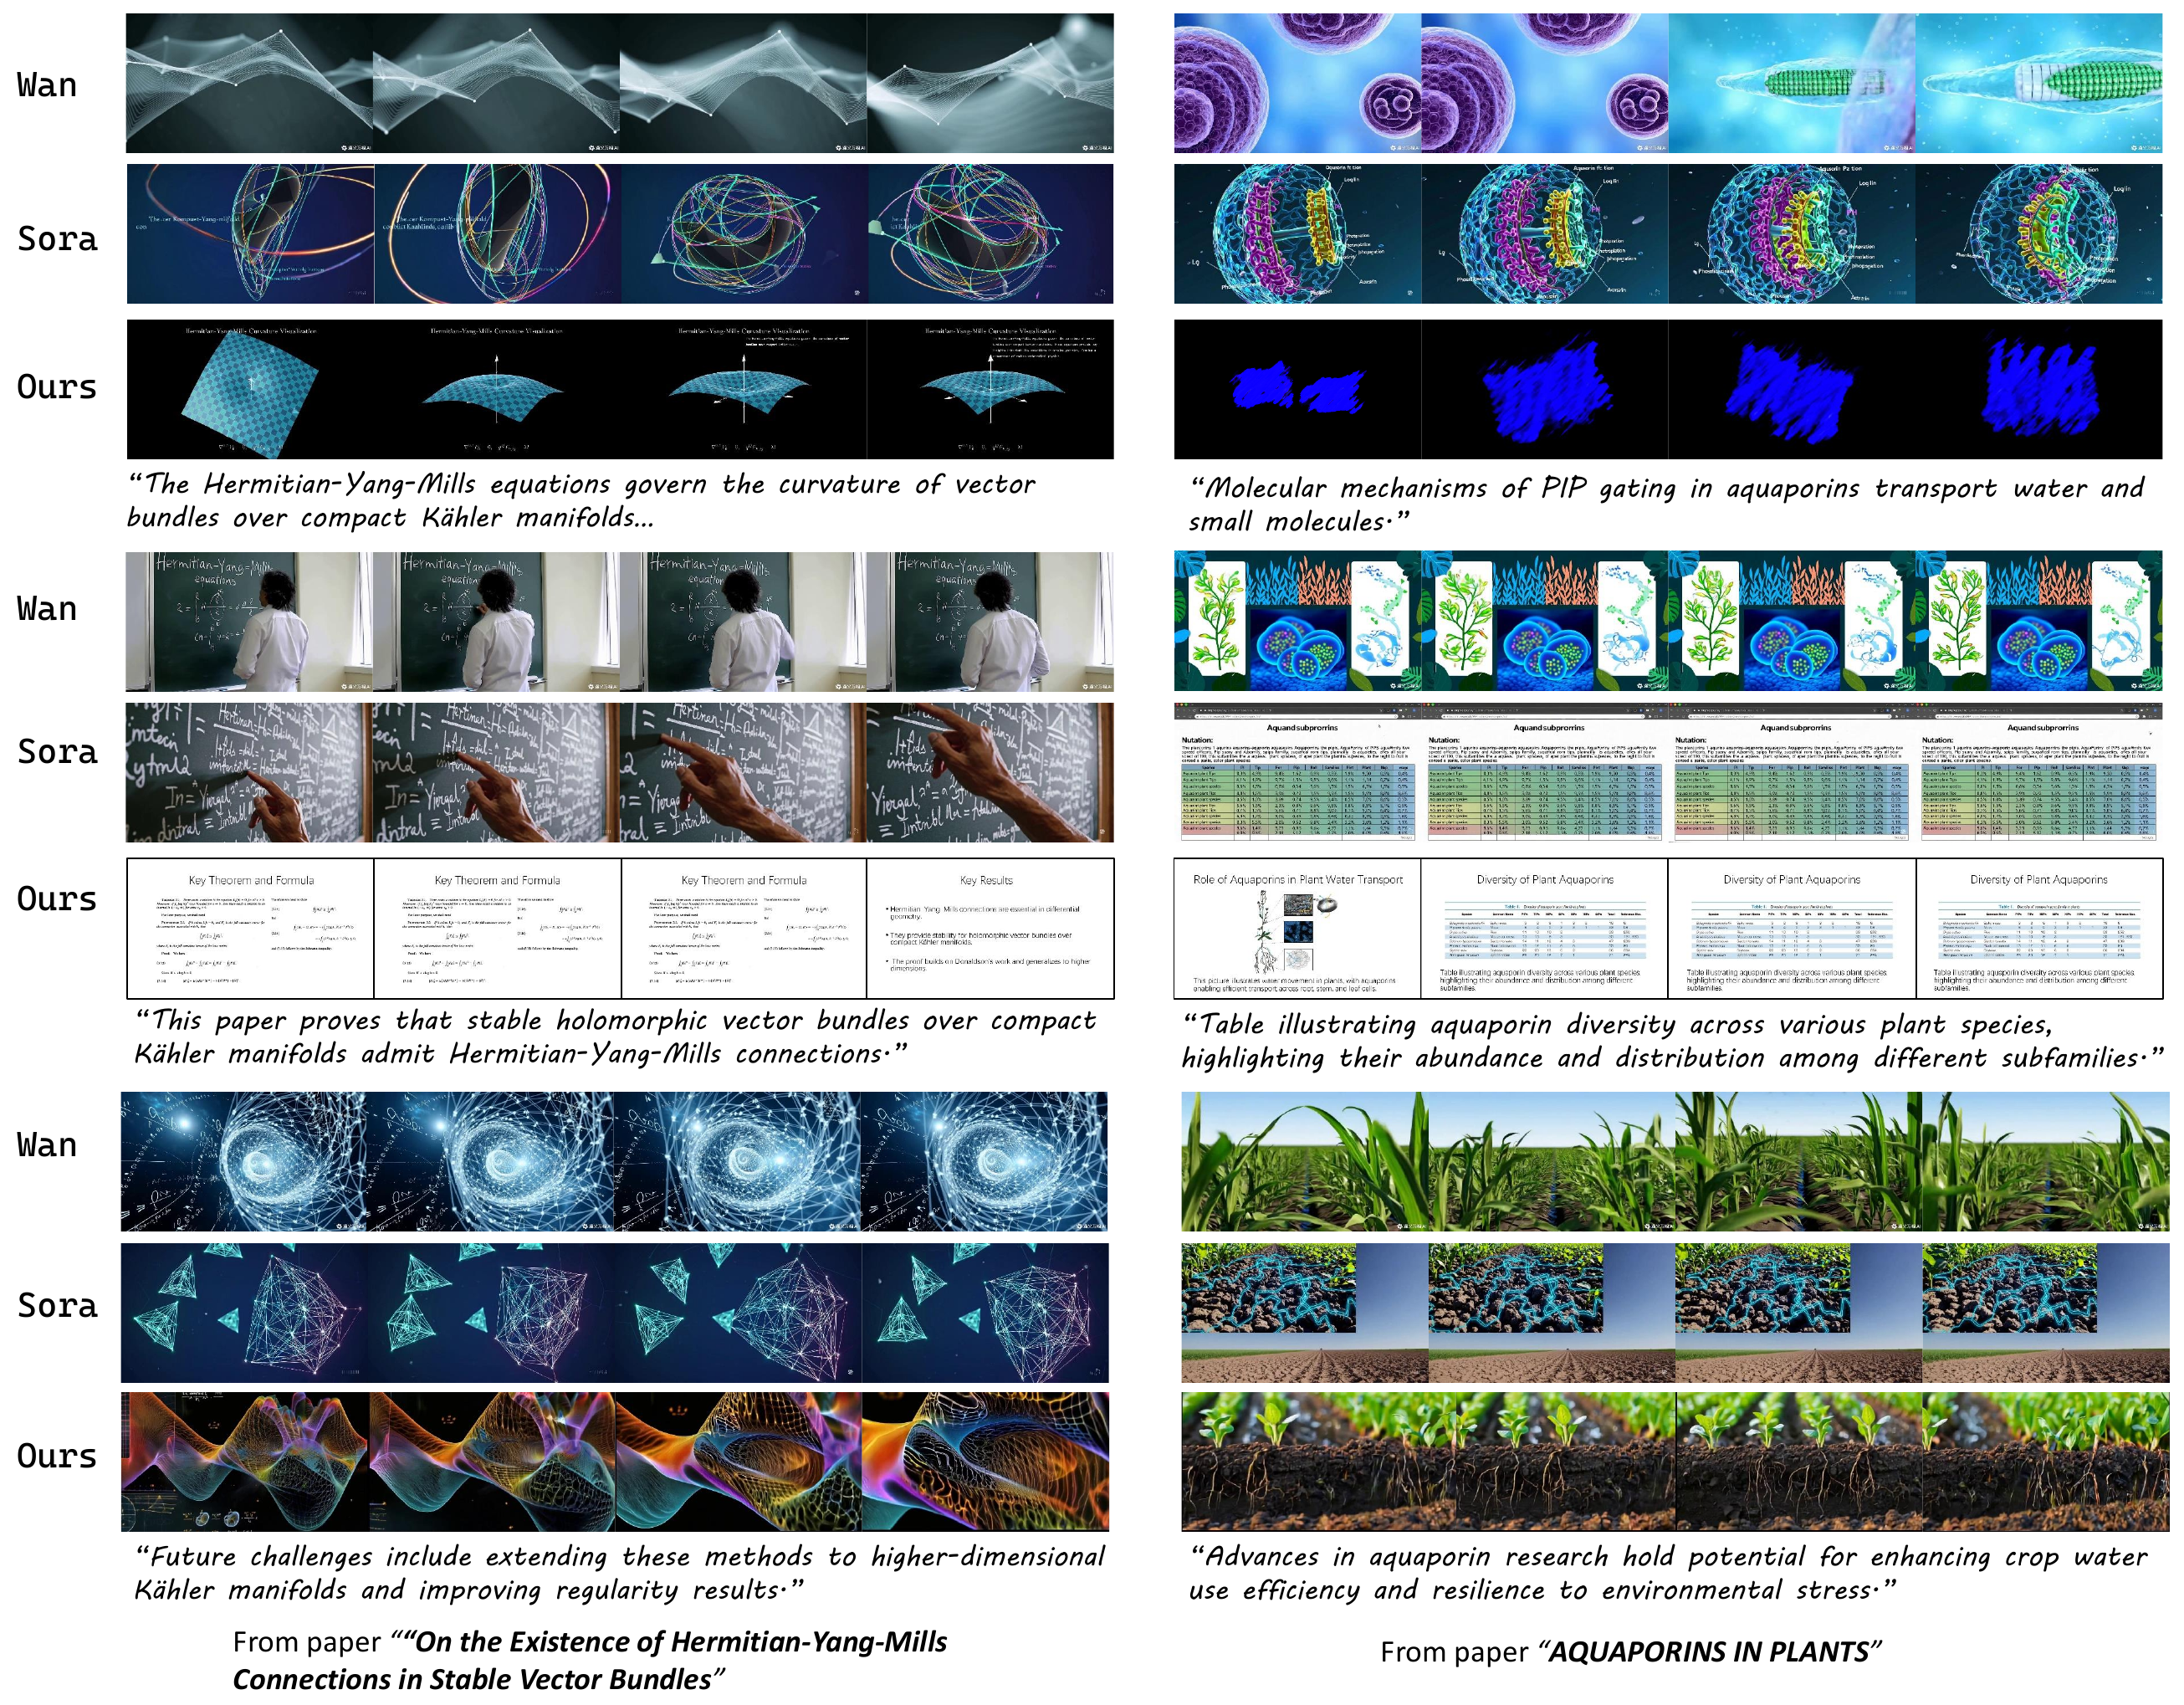}
\vspace{-0.07in}
\caption{The workflow of Preacher. The parts within the dashed box correspond to the process of generating a video segment. If the number of key scenes is $N$ scenes, the process within the dashed box will repeat $N$ times until all video segments are generated. Finally, all the video segments are concatenated as the video abstract.}
% \vspace{-0.17in}
\label{fig:appshow}
\end{figure*}

%\section{Limitations}As the first method to successfully accomplish the paper-to-video task, Preacher still has several limitations. First, given that the approach relies on the collaboration of multiple agents, completing the entire process end-to-end requires over an hour and incurs substantial token consumption for inter-agent communication. Second, the current lack of high-fidelity text-to-animation generation models constrains Preacher's capability to produce animation-style content, limiting its versatility in visual representation. Lastly, when processing papers from research fields like artificial intelligence, the key scenes will exclusively feature the "slides" and "talking heads" styles. This tendency arises from the inherent nature of such papers, which often lack concrete visualizable concepts and instead consist primarily of methodological explanations and experimental analyses.
